# Supplementary material for: Reducing Property Graph Queries to Relational Algebra for Incremental View Maintenance
Source: arXiv:1806.07344 source file (2018-06-19)
Supplement: Supplementary file 1 [file appendix.tex]

\clearpage
\appendix

\section{Foundations of Incremental View Maintenance}

This section is based on~\cite{BergmannPhD} and our earlier publication~\citeself{PerPolQueryOptimization}.

\subsection{Unary Nodes}

\emph{Unary nodes}
have one input slot. They filter or transform the tuples of the parent node according to certain criteria. In the following, the relation representing the input tuples is denoted with $r$, the relation representing the output tuples is denoted with $t$, and the operator processing the input is denoted with $\alpha$:
\begin{align*}
t = \op{\alpha}{r}.
\end{align*}

\paragraph{Maintenance.} In the following, we assume that the $\alpha$ operator is \emph{distributive} \wrt the union ($\union$) and set minus ($\setminus$) operators. If a unary node receives an update $\Delta r$, it performs the operation and computes the change set. For \emph{positive updates}, the result ($t'$) and the changeset ($\Delta t$) are:
\begin{align*}
t'       & \equiv \op{\alpha}{r \union \Delta r} \\
& = \op{\alpha}{r} \union \op{\alpha}{\Delta r} \\
& = t \union \underbrace{\op{\alpha}{\Delta r}}_{\Delta t} \\
\end{align*}

Similarly, for \emph{negative updates}:
\begin{align*}
t'       & \equiv \op{\alpha}{r \setminus \Delta r} \\
& = \op{\alpha}{r} \setminus \op{\alpha}{\Delta r} \\
& = t \setminus \underbrace{\op{\alpha}{\Delta r}}_{\Delta t}
\end{align*}

Unary nodes are often implemented as \emph{stateless} nodes, \ie they do not store the results of the previous executions. Instead, these results are cached in their subscribers, \eg indexers of \emph{binary nodes} (\autoref{sec:binary-nodes}) or \emph{production nodes} (\autoref{sec:production-node}).

As their name suggests, unary nodes implement unary relational algebraic operators (\autoref{sec:unary}):

\begin{itemize}
	\item The \emph{projection node} performs a projection operation on the input relation.
	\item The \emph{selection node} performs a selection operation on the input relation.
\end{itemize}

As both the projection and the selection operators are distributive \wrt the union and set minus operators, their results can be maintained by performing the operation for the change set $\Delta r$.

\subsection{Binary Nodes}
\label{sec:binary-nodes}

\emph{Binary nodes}
have two input slots: the \emph{primary} ($p$) and the \emph{secondary} ($s$). Binary node implementations typically cache both their input relations in \emph{indexers}.

\subsubsection{Natural Join Node}

\paragraph{Maintenance.} In the following, we define the maintenance operations for natural join nodes. If a natural join node receives a \emph{positive update} $\Delta p$ on its \emph{primary} input slot, the result ($t'$) and the change set ($ \Delta t$) are determined as follows:
\begin{align*}
t'       & \equiv \left(p \cup \Delta p\right) \join s           \\
& = (p \join s) \union (\Delta p \join s) \\
& = t \union \underbrace{(\Delta p \join s)}_{\Delta t}
\end{align*}

If the node receives a \emph{positive update} $\Delta s$ on its \emph{secondary} input slot, the result ($t'$) and the change set ($ \Delta t$) are the following:
\begin{align*}
t'       & \equiv p \join \left(s \cup \Delta s\right)           \\
& = (p \join s) \union (p \join \Delta s) \\
& = t \union \underbrace{(p \join \Delta s)}_{\Delta t}
\end{align*}

For \emph{negative updates}, the changeset is the same, but it is propagated as a \emph{negative update}. The result is $t' = t \setminus (\Delta p \join s)$ and $t' = t \setminus (p \join \Delta s)$, for updates messages on the primary and the secondary input slots, respectively.

\subsubsection{Antijoin Node}

\paragraph{Maintenance.} As the antijoin operator is not commutative, handling update messages requires us to distinguish between the following cases:

\begin{itemize}
	\item Update on the primary slot.
	\begin{itemize}
		\item Positive update: send a \emph{positive update} for each incoming tuple for which there is no match on the secondary indexer.
		\begin{align*}
		t'       & \equiv \left(p \cup \Delta p\right) \antijoin s               \\
		& = (p \antijoin s) \union (\Delta p \antijoin s) \\
		& = t \union \underbrace{(\Delta p \antijoin s)}_{\Delta t}
		\end{align*}
		
		\item Negative update: send a \emph{negative update} with the following tuples:
		$$ \Delta t = \Delta p \antijoin s $$
	\end{itemize}
	
	\item Update on the secondary slot. This case is more difficult to handle, so we recall the definition of the antijoin operator from \autoref{sec:binary} for relations $p$ and $s$:
	\begin{align*}
	t & \equiv p \antijoin s = p \setminus \left(p \join \pi_{P \cap S} (s)\right),
	\end{align*}

	\begin{itemize}
		\item For positive updates, the result set can be expressed as:
		\begin{align*}
		t'       & \equiv p \antijoin \left(s \cup \Delta s\right) \\
		& = p \setminus \left( p \join \pi_{P \cap S} \left(s \cup \Delta s\right) \right)
		\end{align*}
		
		Positive updates on the secondary indexer result in \emph{negative updates} on the result set, so that $t' = t \setminus \Delta t$, hence $\Delta t = t \setminus t'$.
		
		For sets $A, B \subseteq C$, the following equality holds: $(C \setminus A) \setminus (C \setminus B) = B \setminus A$.
		Applying this with $C = p$ and using the distributive property of the natural join operator, the change set can be determined as:
		\begin{align*}
		\Delta t = t \setminus t' & = \overbrace{\left[p \setminus \left(p \join \pi_{P \cap S} (s)\right)\right]}^{t} \setminus \overbrace{\left[p \setminus \left( p \join \pi_{P \cap S} \left(s \cup \Delta s\right) \right)\right]}^{t'} \\
		& = \left( p \join \pi_{P \cap S} \left(s \cup \Delta s\right) \right) \setminus \left(p \join \pi_{P \cap S} (s)\right) \\
		& = p \join \left(\pi_{P \cap S} (s \cup \Delta s) \setminus \pi_{P \cap S} (s) \right) \\
		& = p \join \left(\pi_{P \cap S} (s) \cup \pi_{P \cap S} (\Delta s) \setminus \pi_{P \cap S} (s) \right) \\
		& = p \join \left(\pi_{P \cap S} (\Delta s) \setminus \pi_{P \cap S} (s) \right)
		\end{align*}
		
		\item For negative updates, the result set can be expressed as:
		\begin{align*}
		t' & \equiv p \antijoin \left(s \setminus \Delta s\right) \\
		& = p \setminus \left(p \join \pi_{P \cap S} \left(s \setminus \Delta s\right)\right),
		\end{align*}
		
		Negative updates may result in \emph{positive updates} on the result set. Since $t' = t \union \Delta t$, we can define $\Delta t = t' \setminus t$:
		\begin{align*}
		\Delta t = t' \setminus t & = \overbrace{\left[p \setminus \left( p \join \pi_{P \cap S} \left(s \setminus \Delta s\right) \right)\right]}^{t'} \setminus \overbrace{\left[p \setminus \left(p \join \pi_{P \cap S} (s)\right)\right]}^{t} \\
		& = \underbrace{\left(p \join \pi_{P \cap S} (s)\right)}_{x} \setminus \underbrace{\left( p \join \pi_{P \cap S} \left(s \setminus \Delta s\right) \right)}_{y}
		\end{align*}
		Although this change set may seem difficult to calculate, we point out that both $x$ and $y$ can be maintained incrementally. Furthermore, they only grow linearly in the size of $p$, as the join operator does not introduce new attributes, hence it can only reduce the number of elements in the relation.
	\end{itemize}
\end{itemize}

\subsection{Production Nodes}
\label{sec:production-node}

\emph{Production nodes} are terminators that provide an interface for fetching results of a query (the match set) and also propagate the changes introduced by the latest update message.\footnote{In popular Rete implementations, clients are usually subscribed to the production nodes and notified about the changes in the result set.}

\paragraph{Maintenance.} The change set is defined as:
$$\Delta t \equiv \bigcup_{i=1}^{n} \Delta r_i,$$

where $\Delta r_1, \Delta r_2, \ldots, \Delta r_n$ are the update messages triggered by the last change.
